# Supplementary material for: Representation Learning for Frequent Subgraph Mining
Source: arXiv:2402.14367 source file (2024-02-22)
Supplement: Supplementary file 1 [file 060appendix.tex]

\appendix

\section{Proofs of Subgraph Properties}
NeuroMatch~\cite{neuralsubgraphmatching} introduces the following observations that demonstrate the natural use of order embeddings in subgraph matching.
The arguments hold for both the problem of subgraph matching, and motif mining. We list the correspondences between order embedding and subgraph relation in this section for completeness.

Note, however, that these subgraph relations are not able to account for the appearances of multiple of the same subgraph in the target graph, as required by motif mining. Therefore \name solves this challenge by encoding node neighborhoods in the target graph, and performing a walk in the order embedding space.

\xhdr{Transitivity}
Suppose that $G_1$ is a subgraph of $G_2$ with bijection $f$ mapping all nodes from $G_1$ to a subset of nodes in $G_2$, and $G_2$ is a subgraph of $G_3$ with bijection $g$. 
Let $v_1, v_2, v_3$ be anchor nodes of $G_1, G_2, G_3$ respectively.
By definition of anchored subgraph, $f(v_1) = v2$ and $g(v_2) = v_3$.
Then the composition $g \circ f$ is a bijection.
Moreover, $g\circ f (v_1) = g(v_2) = v_3$, where  Therefore $G_1$ is a subgraph of $G_3$, and thus the transitivity property.

This corresponds to the transitivity of order embedding.

\xhdr{Anti-symmetry}
Suppose that $G_1$ is a subgraph of $G_2$ with bijection $f$, and $G_2$ is a subgraph of $G_1$ with bijection $g$.
Let $|V_1|$ and $|V_2|$ be the number of nodes in $G_1$ and $G_2$ respectively. By definition of subgraph isomorphism, $G_1$ is a subgraph of $G_2$ implies that $|V_1| \le |V_2|$. Similarly, $G_2$ is a subgraph of $G_1$ implies $|V_2| \le |V_1|$.
Hence $|V_1| = |V_2|$. The mapping between all nodes in $G_1$ and $G_2$ is bijective. By definition of isomorphism, $G_1$ and $G_2$ are graph-isomorphic.

This corresponds to the anti-symmetry of order embedding.

\xhdr{Intersection}
By definition, if $G_3$ is a common subgraph of $G_1$, $G_2$, the $G_3$ is a subgraph of both $G_1$ and $G_2$. Since a trivial node is a subgraph of any graph, there is always a non-empty intersection set between two graphs.

Correspondingly, if $z_3 \preceq z_1$ and $z_3 \preceq z_2$, then $z_3 \preceq \min \{ z_1, z_2\}$.
Here $\min$ denotes the element-wise minimum of two embeddings. Note that the order embedding $z_1$ and $z_2$ are positive, and therefore $\min \{ z_1, z_2\}$ is another valid order embedding, corresponding to the non-empty intersection set between two graphs.

Note that this paper assumes the frequent motifs are connected graphs.
And thus it also assumes that all neighborhoods in a given datasets are connected and contain at least 2 nodes (an edge). 
This is a reasonable assumption since we can remove isolated nodes from the datasets, as connected motifs of size $k$ ($k>1$) can never contain isolated nodes.
In this case, the trivial intersection corresponds to a graph of 2 nodes and 1 edge. 

\section{Model Analysis}

\subsection{Proof of order embedding expressiveness}
\begin{proposition}
Given a graph dataset of size $n$, we can find a perfect order embedding of dimension $D$, where $D$ is the number of non-isomorphic node-anchored graphs of size no greater than $n$. The perfect order embeddings satisfy $z(G_Q) \preceq z(G)$ if and only if $G_Q$ is a subgraph of $G$.
\end{proposition}

\begin{proof}
This perfect order embedding can be simply constructed by enumerating all possible non-isomorphic node-anchored graphs of size no greater than $n$, and place the count of the $i$-th graph into the $i$-th dimension of the order embedding.

If graph $G_Q$ is a subgraph of graph $G$, then by definition there exists an isomorphism $f$ between $G_Q$ and a subgraph of $G$. Therefore each motif in $G_Q$ can be mapped to the corresponding motif in $G$ by $f$. Hence the motif count of $G_Q$ for any motif is no less than the corresponding motif count of $G$.

Conversely, if graph $G_Q$ is not a subgraph of graph $G$, then the motif isomorphic to $G_Q$ has count at least $1$ for $G_Q$, and $0$ for graph $G$, violating the order constraint. 
\end{proof}

\subsection{Motif Counts Prediction}
As an experiment to demonstrate the capability of GNNs in predicting motif counts, we randomly generate graphs using synthetic and real datasets \cite{KKMMN2016} and train a GNN to predict (log) counts of small motifs, as computed by exact enumeration. We find that GNNs are able to accurately estimate these counts, with relative mean squared error of around 10\% across all datasets. Together with Proposition 1, this finding confirms their capacity to learn order embeddings that capture the subgraph relation.

\begin{table}[t]	
\centering
\resizebox{0.9\linewidth}{!}{
\begin{tabular}{clccccc}\cmidrule[\heavyrulewidth]{2-7}
& \textbf{Dataset} &\multicolumn{1}{c}{\textsc{E-R}} & \multicolumn{1}{c}{\textsc{COX2}} & \multicolumn{1}{c}{\textsc{DD}} & \multicolumn{1}{c}{\textsc{\textsc{MSRC\_21}}} & \multicolumn{1}{c}{\textsc{FirstMMDB}}  
%&  \multicolumn{1}{c}{\textsc{PPI}} & \multicolumn{1}{c}{\textsc{WordNet18}} 
\\ 
\cmidrule{2-7}
& \textsc{MSE} & 8.4  & 7.1  &  8.9  &  10.5  & 12.7    \\ 
& \textsc{Rel Err} & 9.4\%  & 12.5\%  &  11.8\%  &  13.4\%  & 11.5\% \\ 
\cmidrule[\heavyrulewidth]{2-7}
\end{tabular}}
\caption{The MSE and relative MSE for predicting log of motif counts.}
\label{tab:all_match_AUROC}
\end{table}

\section{Further Implementation Details}

\xhdr{Synthetic dataset}
We design a synthetic graph generator to provide training graphs for synthetic pretraining, so that the model learns an order embedding space over diverse types of graphs and can generalize to new datasets at inference time.

We design a generator that randomly chooses one of the following generators:
Erd\H{o}s-R\'enyi (E-R)~\cite{erdds1959random}, Extended Barabási–Albert graphs~\cite{albert2000topology}, Power Law Cluster graphs~\cite{holme2002growing} and Watts-Strogatz graph~\cite{watts1998collective}. We design prior distributions for the parameters for each of the generators. For the Erd\H{o}s-R\'enyi generator, the probability of an edge is $p \sim \textrm{Beta}(1.3, 1.3n/\log_2(n) - 1.3)$. For the Extended Barabási–Albert generator, the number of attachment edges per node is $m \sim \textrm{Unif}(1, 2\log_2 n)$, the probability of adding edges is $p \sim \textrm{Exp}(20)$ (capped at $0.2$) and the probability of rewiring edges is $q \sim \textrm{Exp}(20)$ (capped at $0.2$). For the Power Law Cluster generator, the number of attachment edges per node is $m \sim \textrm{Unif}(1, 2\log_2 n)$ and the probability of adding a triangle after each edge is $p \sim \textrm{Unif}(0, 0.5)$. For the Watts-Strogatz generator, each node is connected to $k \sim n\textrm{Beta}(1.3, 1.3n/\log_2(n) - 1.3)$ neighbors (minimum $2$) and the rewiring probability is $p \sim \textrm{Beta}(2, 2)$. Here $n$ is the desired graph size.

% Using this graph generator, we create a balanced dataset of graph pairs $(A, B)$ in which a pair is positive if $B$ is a subgraph of $A$. To create positive pairs, we sample a graph $A$ from the generator and sample a subgraph $B$ using the sampling procedure of \textsc{MFinder}~\cite{kashtan2004efficient}. To create negative pairs, we sample a graph $A$ from the generator. With 50\% probability, we sample a subgraph $B$ as in the positive case, then randomly add up to 5 edges to $B$ so that it is unlikely to be a subgraph of $A$. Otherwise, we sample an auxilliary subgraph $X$ of the same size as $A$, then let $B$ be a sampled subgraph of $X$, making it unlikely to be a subgraph of $A$. We sample $A$ of size uniform from 6 to 29 and $B$ of size uniform from 5 to $|A|-1$.

\xhdr{Dataset statistics}
We demonstrate that our synthetic data generation scheme is capable of generating graphs with high variety. Figure \ref{fig:syn-real-stats} shows the statistics of the synthetic graphs, compared to real-world datasets. In terms of graph statistics, including density, diameter, average shortest path length, and average clustering coefficient, the synthetic dataset (large blue dots) covers most of the real-world datasets, including those in the domains of chemistry (\textsc{COX2}), biology (\textsc{ENZYMES}) and social networks (\textsc{Reddit-Binary}) \cite{Fey/Lenssen/2019}.

The high coverage of statistics suggests that the synthetic dataset can serve well as a application-agnostic dataset that allows our model \name to learn order embedding models in the most generic sense. 
In practice, given a very small real-world dataset, one can train on this synthetic dataset, and transfer the model (either directly or with fine-tuning) to apply to this real-world dataset.

\xhdr{Training details} 
Our encoder model architecture consists of a single hidden-layer feedforward module, followed by 8 graph convolutions with ReLU activation and learned dense skip connections, followed by a 4-layer perceptron with 64-dimensional output. We use SAGE graph convolutions \cite{hamilton2017inductive} with sum aggregation and no neighbor sampling. We train the network with the Adam optimizer using learning rate $10^{-4}$ for 1 million batches of synthetic data, with batch size 64 and balanced class distribution.

\xhdr{Decoder configuration}
To sample node-anchored neighborhoods, we follow the iterative procedure of \textsc{MFinder}~\cite{kashtan2004efficient}: after picking a random node as the anchor, we maintain a search tree, in each step randomly picking a node from the frontier with probability weighted by its number of edges with nodes in the search tree. The procedure terminates when the search tree reaches $N$ nodes, and we take the subgraph induced by these nodes as the neighborhood. We select $N$ uniformly randomly from 20 to 29 for each neighborhood (except for Experiment \textbf{(2)}, where the maximum size is 25), sampling 10000 neighborhoods in total.

For a given maximum motif size $k$, \name generates all motifs up to size $k$ through a single run of the search procedure. For the greedy procedure, we sample 1000 seed nodes and expand each corresponding candidate motif up to size $k$, recording all candidates for intermediate sizes. For the MCTS procedure, we run a total of 1000 simulations, divided equally among each motif size up to $k$, reusing the existing search tree with each new iteration; this procedure creates a useful prior for each successive motif size. We use exploration constant $c=0.7$ throughout.

\xhdr{Baseline configuration}
For \textsc{MFinder} \cite{kashtan2004efficient}, we sample 10000 neighborhoods per motif size. We omit the slow $O(n^{n+1})$ exact probability correction, simply weighting each sampled neighborhood equally. We take the first sampled node as the anchor node in node-anchored experiments.

For \textsc{Rand-ESU} \cite{wernicke2006efficient}, we set the expansion probabilities for each search tree level $i$ according to $p_i = (1-i/(k+1))^\tau$ where $k$ is the maximum motif size and $\tau$ can be tuned for runtime depending on the dataset; we use $\tau=5$ for \textsc{Enzymes} (except $\tau=2.3$ in Experiment \textbf{(1)}), $\tau=2$ for \textsc{Cox2}, $\tau=2$ for \textsc{MNRoads} and $\tau=9$ for \textsc{Coil-Del}. We use the suggested variance reduction technique of sampling a fixed proportion of children to expand at each level.

For both methods, we use the WL-isomorphism test to count motif frequencies.

\section{Further Experimental Results}

\xhdr{Extended planted motif results}
Figure \ref{fig:extra_planted_motif_results} shows the full set of top ten subgraphs identified by \name\ for each planted motif in Experiment \textbf{(2)}. In three of the four cases, the planted motif is the top-ranked motif identified by the model. Note that the model tends to identify subgraphs similar to the planted motif, though often with additional ``attachment edges''; motifs with these attachments tend to be frequent as well due to the dataset construction.

\begin{figure*}[t]
    \centering
    \includegraphics[width=0.95\textwidth]{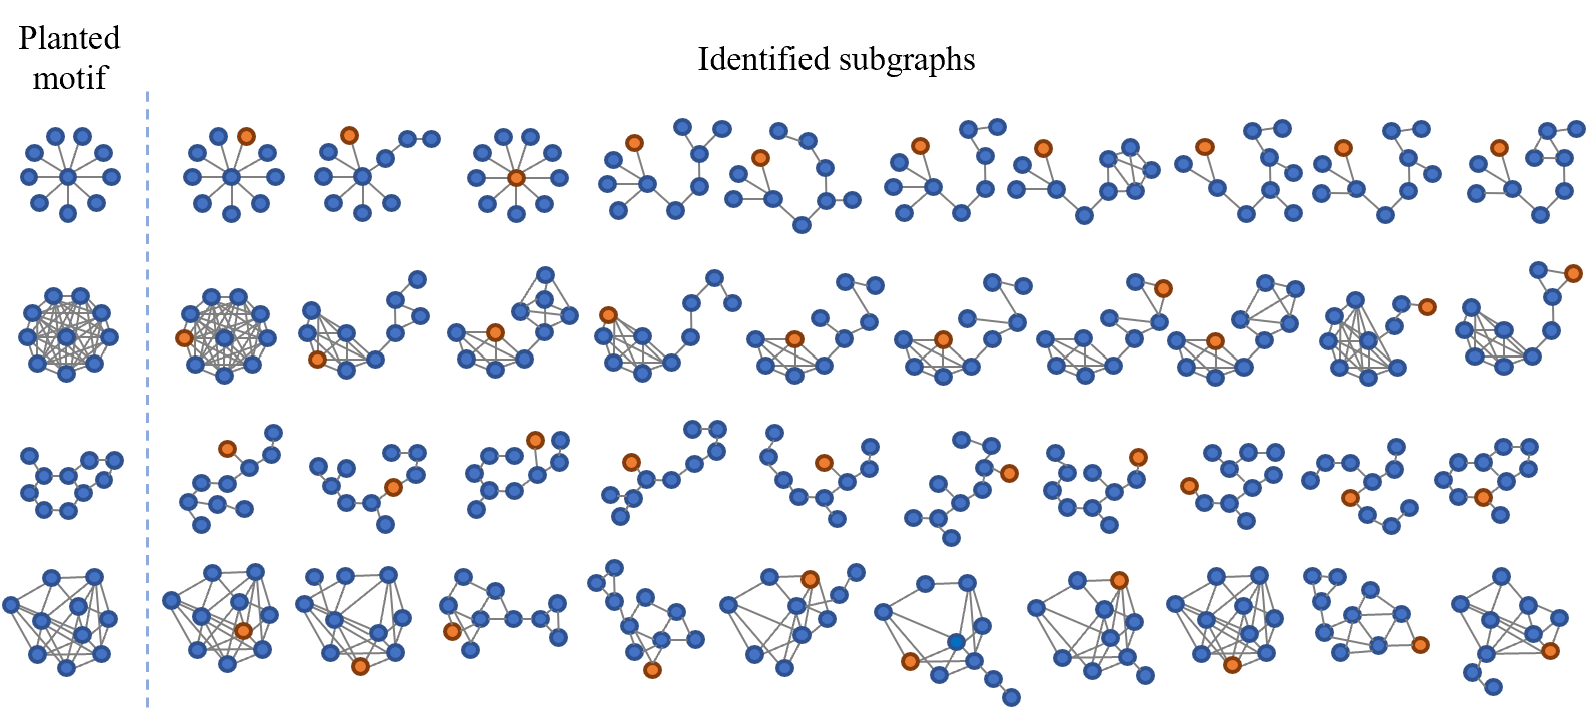}
    \caption{Full set of top ten subgraphs identified by \name\ for each planted motif, ordered by increasing rank from left to right. In three of the four cases, the planted motif is the top-ranked motif identified by the model. Anchor nodes are shown in orange.}
    \label{fig:extra_planted_motif_results}
\end{figure*}

\xhdr{Frequency comparison of identified motifs}
We additionally run Experiment \textbf{(3)} on two more datasets, \textsc{Coil-Del}~\cite{riesen2008iam}, a dataset of 3D objects derived from COIL-100, and a graph of the Minnesota road network ~\cite{netrepo}, abbreviated \textsc{MNRoads}. We find again that \name\ consistently identifies more frequent motifs than the baselines, especially for large graphs (Figure \ref{fig:extra_freq_comparison}).
\begin{figure}
    \centering
    \includegraphics[width=0.4\textwidth]{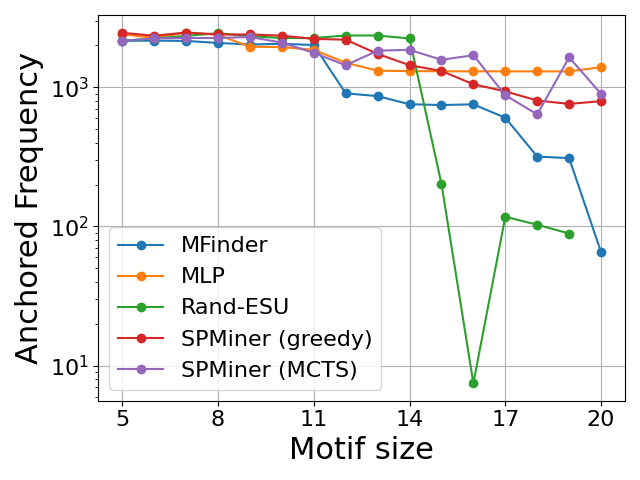}
    \hspace{1cm}
    \includegraphics[width=0.4\textwidth]{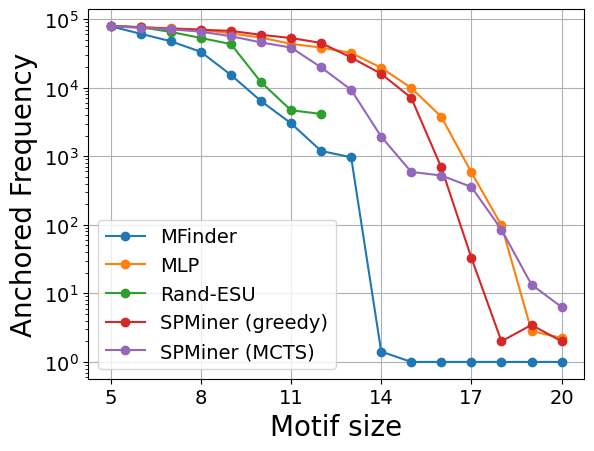}
    \caption{Median frequencies of motifs identified by \name and baselines for each graph size; higher is better. Left: \textsc{MNRoads}; right: \textsc{Coil-Del}.}
    \label{fig:extra_freq_comparison}
\end{figure}

\section{Runtime Comparison}
\xhdr{Runtime comparison with approximate methods}
We tune the hyperparameters so that all methods are comparable in runtime and sample a comparable number of subgraphs. All methods are single-process and implemented with Python; the neural methods are implemented with PyTorch Geometric~\cite{Fey/Lenssen/2019}. We run all methods on a single Xeon Gold 6148 core; the neural methods additionally use a single Nvidia 2080 Ti RTX GPU. Table \ref{tab:runtime_comparison} shows that \name\ both runs in less time and requires fewer subgraph samples than the baselines.

\xhdr{Runtime comparison with exact methods}
In experiments, we compare with exact methods gSpan~\cite{yan2002gspan} and Gaston~\cite{nijssen2005gaston}. For gSpan, we use a highly optimized C++ implementation\footnote{\url{https://github.com/Jokeren/gBolt}}, which we modify to prune the search once the identified motif reaches the specified maximum motif size, in order to increase its efficiency in our setting. We use the single-threaded version. For Gaston, we use the official C++ implementation\footnote{\url{http://liacs.leidenuniv.nl/~nijssensgr/gaston/download.html}}, using the variant with occurrence lists and specifying the desired maximum motif size through a command-line argument. We impose a resource limit of two hours of runtime and 50GB of memory for both methods. We run both methods on a single Xeon Gold 6148 core.

%\xhdr{gSpan and Gaston objective}
%The previous exact methods including gSpan and Gaston focuses on a slightly different frequency definition than Defintion 1 and 2 in this work. They assume that a graph dataset has to contain multiple graphs, and define motif frequency as the nubmer of graphs in the dataset containing the motif. 

\begin{table*}[t]
    \centering
\begin{tabular}{cc}
    \begin{subtable}[t!]{0.45\textwidth}
        \centering
        \resizebox{\linewidth}{!}{
        \begin{tabular}[t!]{clcccc}\cmidrule[\heavyrulewidth]{2-6}
        & \textbf{Dataset} &\multicolumn{1}{c}{\textsc{Enzymes}} & \multicolumn{1}{c}{\textsc{COX2}} & \multicolumn{1}{c}{\textsc{COIL-DEL}} & \multicolumn{1}{c}{\textsc{MNRoads}} 
        %&  \multicolumn{1}{c}{\textsc{PPI}} & \multicolumn{1}{c}{\textsc{WordNet18}} 
        \\ 
        \cmidrule{2-6}
                    & \textsc{Rand-ESU} & 13:59 & 13:56 & 19:22 & 4:47 \\
                    & \textsc{MFinder} & 17:29 & 17:13 & 20:57 & 16:24 \\
                    & \name & 9:26 & 8:13 & 11:15 & 9:41 \\
        \cmidrule[\heavyrulewidth]{2-6}
        \end{tabular}}
        \caption{Runtime comparison with approximate methods}
    \end{subtable}
&
    \begin{subtable}[t!]{0.45\textwidth}
        \centering
        \resizebox{\linewidth}{!}{
        \begin{tabular}[t!]{clcccc}\cmidrule[\heavyrulewidth]{2-6}
        & \textbf{Dataset} &\multicolumn{1}{c}{\textsc{Enzymes}} & \multicolumn{1}{c}{\textsc{COX2}} & \multicolumn{1}{c}{\textsc{COIL-DEL}} & \multicolumn{1}{c}{\textsc{MNRoads}} 
        %&  \multicolumn{1}{c}{\textsc{PPI}} & \multicolumn{1}{c}{\textsc{WordNet18}} 
        \\ 
        \cmidrule{2-6}
                    & \textsc{Rand-ESU} & 39235 & 29368 & 85149 & 7605 \\
                    & \textsc{MFinder} & 10000 & 10000 & 10000 & 10000 \\
                    & \name & 1500 & 1500 & 1500 & 1500 \\
        \cmidrule[\heavyrulewidth]{2-6}
        \end{tabular}}
        \caption{Average number of subgraphs sampled}
    \end{subtable}
    \end{tabular}
    \caption{Comparison of runtimes and number of  subgraphs sampled (averaged over all motif sizes) for each method in Experiment \textbf{(3)}. \textsc{SPMiner} has the lowest runtimes and requires fewer samples to identify frequent motifs. We compare against the greedy variant of \name; the MCTS variant samples the same number of subgraphs and incurs small computational overhead.}
    \label{tab:runtime_comparison}
\end{table*}

\section{GNN expressive power}
Previous works~\cite{xu2018how,morris2019weisfeiler} have identified limitations of a class of GNNs. More specifically, GNNs face difficulties when asked to distinguish regular graphs. 
In this work, we circumvent the problem by distinguishing the anchor node and other nodes in the neighborhood via one-hot encoding (See Section 3.2). The idea is explored in a concurrent work ``Identity-aware Graph Neural Networks'' (ID-GNNs). It uses Figure \ref{fig:overview} to demonstrate the expressive power of ID-GNN, which distinguishes anchor node from other nodes. For example, while d-regular graphs such as 3-cycle and 4-cycle graphs have the same GNN computational graphs, their ID-GNN computational graphs are different, due to identification of anchor nodes via node features.
Such modification enables better expressive power than message-passing GNNs such as GIN.

A future direction is to investigate the performance of recently proposed more expressive GNNs~\cite{chen2019equivalence} in the context of subgraph mining.
The \name framework is general and any GNN can be used in its decoder component, and could benefit from more expressive GNNs.
\begin{figure*}[t]
\centering
\includegraphics[width=0.95\linewidth]{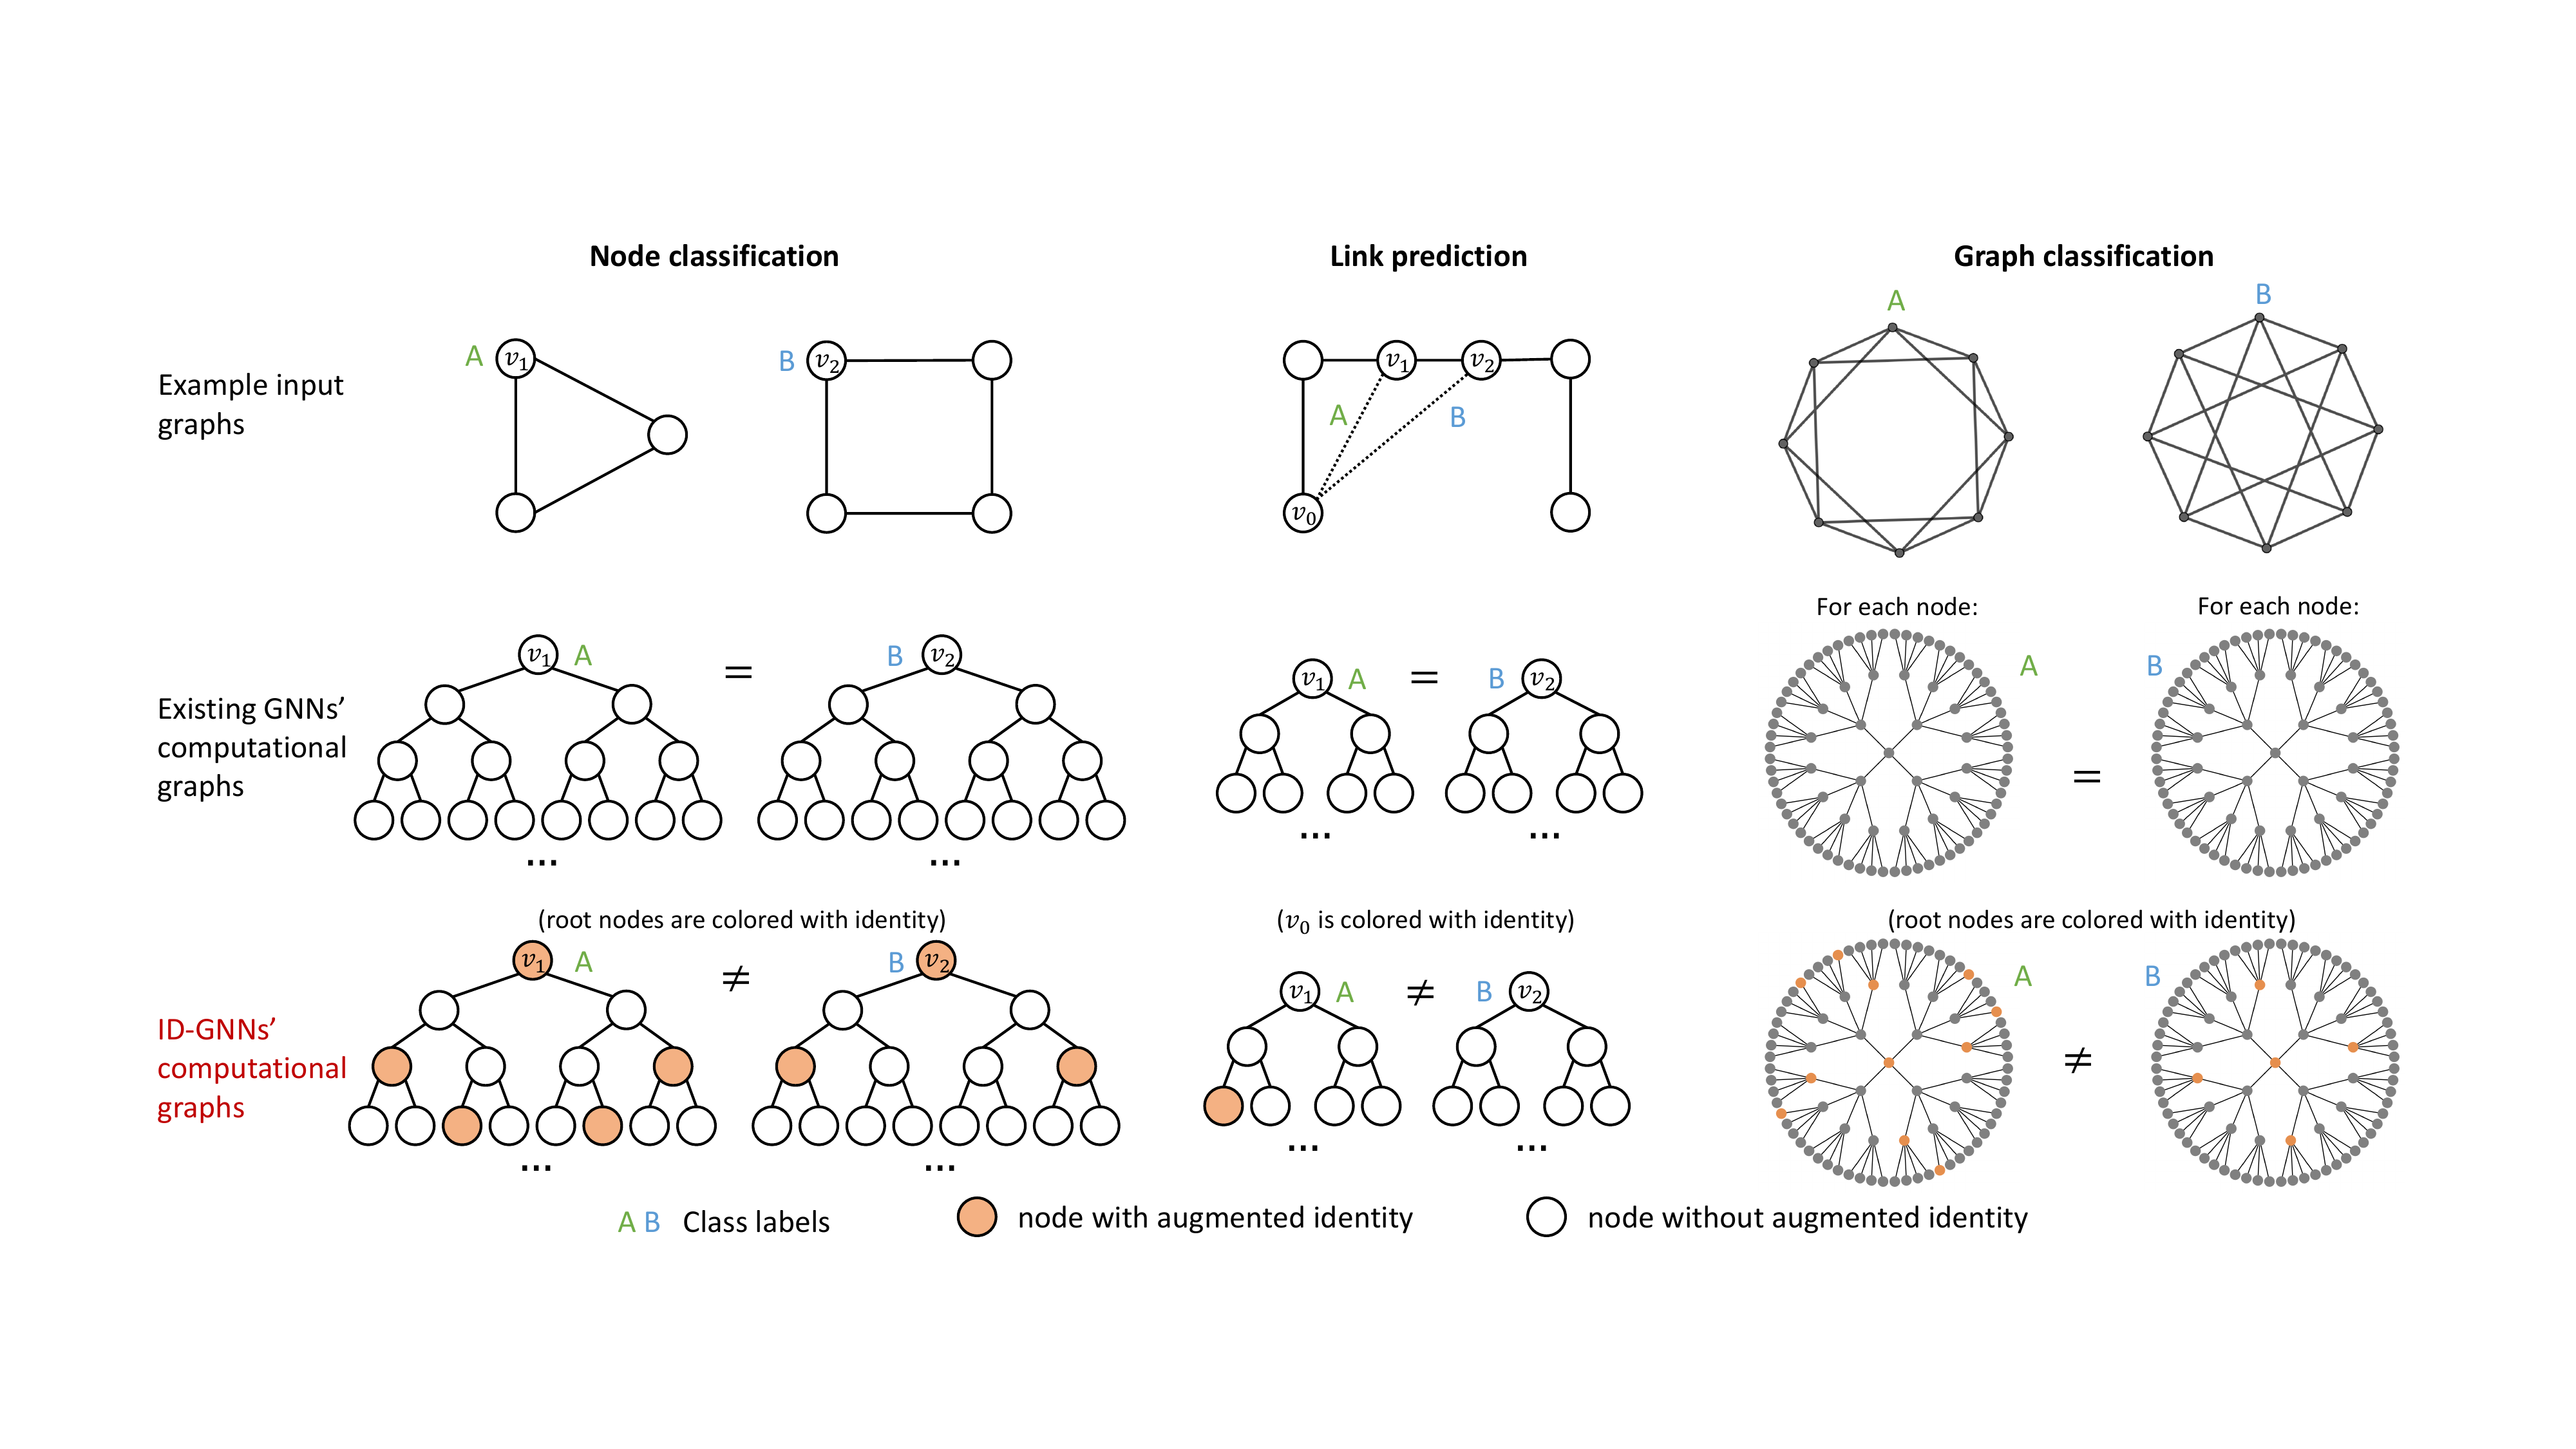} 
\vspace{-2mm}
\caption{
An overview of the proposed ID-GNN model. 
We consider node, edge and graph level tasks, and assume nodes do not have additional features.
Across all examples,
the task requires an embedding that allows for the differentiation of the label $A$ vs. $B$ nodes in their respective graphs. However, across all tasks, existing GNNs, regardless of depth, will \textit{always} assign the same embedding to both classes of nodes, because for all tasks the computational graphs are identical. In contrast, the colored computation graphs provided by ID-GNNs allows for clear differentiation between the nodes of class $A$ and class $B$, as the colored computation graph are no longer identical across all tasks.  
\vspace{-5mm}
}
\label{fig:overview}
\end{figure*}
